# Supplementary material for: Fireiron: A Scheduling Language for High-Performance Linear Algebra on GPUs
Source: arXiv:2003.06324 source file (2020-03-13)
Supplement: Supplementary file 1 [file appendix.tex]

\subsection{Installation}
\begin{enumerate}
        \item Install scala
        \item Install sbt (https://www.scala-sbt.org/)
        \item Install IntelliJ (https://www.jetbrains.com/idea/)
        \item Clone the repository (https://gitlab-master.nvidia.com/rbodik/fireiron)
        \item Check scala and sbt installation: Change into the fireiron directory and run sbt compile
        \item Start Intellij and import the fireiron project.
\end{enumerate}

\subsection{MMA Decompositions}
\begin{figure*}
\begin{lstlisting}[style=fireiron, language=Fireiron, numbers=left]
    Fluent
      /// CTA-level /////////////////////////////////////////////////////////////////////
      .tile(ctaTile.m, ctaTile.n).to(CTA)
      .epilog(RF, FP32,
        //--- init ------------------------------------------------------------------------
        Fluent
          .tile(warpTileM, warpTileN).to(Warp)
          .tile(16, 16).unrollTile
          .tile(2, 4).to(Lane)
          .tile(1, 1).unrollTile.done,
        //--- store results to GL ---------------------------------------------------------
        Fluent
          .load(SplitKReduction.src, SH, Spec
            .tile(warpTileM, warpTileN).to(Warp)
            .split(ctaTile.m) // special care!
            .tile(16, 16).unrollTile
            .apply(hmma884F32TNOwnership)
            .tile(1, 1).unrollTile.done).storeAs(FP16).reuseBuffer
          .tile(ctaTile.m, ctaTile.n / howManyWarps).to(Warp)
          .tile(ctaTile.m, 32 / (ctaTile.m / 8)).unrollTile
          .tile(8, 1).to(Lane).threadLayout(ThreadLayout.ColMajor).done
      ).splitK
      //--- 128x128x32 CTA-block ---------------------------------------------------------
      .split(64).sync.vars("SPLIT").unrollSplit.swizzle(test, test).prefetchLoads
      //--- A: GL -> SH ------------------------------------------------------------------
      // LDG
      .load(MatMul.a, RF, Fluent
        .tile(howManyWarps * 2 * 4, 64).unrollTile
        .tile(4, 64).to(Warp)
        .tile(1, 8).to(Lane).donePtx
      ).align(16).guard(s"${test(Var("SPLIT"))} < (KK / ${ctaTile.k})")
      .load(MatMul.a, SH, Fluent
        // STS
        .tile(howManyWarps * 2 * 4, 64).unrollTile
        .tile(4, 64).to(Warp)
        .tile(1, 8).to(Lane)
        .swizzle(stsSwizzle) //.printSwizzle(stsSwizzleScala)
        .done
      ).noSync.postponed
      //--- B: GL -> SH ------------------------------------------------------------------
      .load(MatMul.b, RF, Fluent
        .tile(64, howManyWarps * 2 * 4).unrollTile
        .tile(64, 4).to(Warp)
        .tile(8, 1).to(Lane).threadLayout(ThreadLayout.ColMajor).donePtx
      ).align(16).guard(s"${test(Var("SPLIT"))} < (KK / ${ctaTile.k})")
      .load(MatMul.b, SH, Fluent
        .tile(64, howManyWarps * 2 * 4).unrollTile
        .tile(64, 4).to(Warp)
        .tile(8, 1).to(Lane).threadLayout(ThreadLayout.ColMajor)
        .swizzle(stsSwizzle) //.printSwizzle(stsSwizzleScala)
        .done).postponed
      /// WARP-level /////////////////////////////////////////////////////////////////////
      .tile(warpTileM, warpTileN).to(Warp)
      .split(32).splitK(Warp)
      //--- XMMA-tile ------------------------------------------------------------------//
      .split(8).unrollSplit.vars("XMMAS_K").swizzle(ldsSwizzle, ldsSwizzle).doubleBufferLoop
      .load(MatMul.a, RF, loadAFragments).doubleBuffer
      .load(MatMul.b, RF, loadBFragments).doubleBuffer
      .tile(16, 16).unrollTile.vars("XMMAS_N", "XMMAS_M")
      //--- _mma-tile ------------------------------------------------------------------//
      /// LANE-level /////////////////////////////////////////////////////////////////////
      .mma // implicitly assigns created chunks to lanes
      .done
\end{lstlisting}
\caption{Fireiron: HMMA In-CTA-split-k.}
\label{fig:splitk}
\end{figure*}

\begin{figure*}
\begin{lstlisting}[style=fireiron, language=Fireiron, numbers=left]
 Fluent
      /// CTA-level /////////////////////////////////////////////////////////////////////
      .tile(ctaTile.m, ctaTile.n).to(CTA)
      .epilog(RF, FP32, // accumulate using FP32
        //--- init ------------------------------------------------------------------------
        Fluent
          .tile(warpTileM, warpTileN).to(Warp)
          .tile(16, 16).unrollTile
          .tile(2, 4).to(Lane)
          .tile(1, 1).unrollTile.done,
        //--- store results to GL ---------------------------------------------------------
        Fluent
          .load(Move.src, SH, Spec
            .tile(warpTileM, warpTileN).to(Warp)
            .tile(16, 16).unrollTile
            .apply(hmma884F32TNOwnership)
            .tile(1, 1).unrollTile.done).storeAs(FP16).reuseBuffer
          .tile(ctaTile.m, ctaTile.n / (warpsM * warpsN)).to(Warp)
          .tile(ctaTile.m, 32 / (ctaTile.m / 8)).unrollTile
          .tile(8, 1).to(Lane).threadLayout(ThreadLayout.ColMajor)
          .done
      )
      //--- 128x128x32 CTA-block ---------------------------------------------------------
      .split(ctaTile.k).sync.vars("SPLIT").unrollSplit.swizzle(test, test).prefetchLoads
      //--- A: GL -> SH ------------------------------------------------------------------
      .load(MatMul.a, RF, Fluent
        .tile(aGmemTile.columnsPerLDG, aGmemTile.contiguous).unrollTile
        .tile(aGmemTile.columnsPerLDGPerWarp, aGmemTile.contiguous).to(Warp)
        .tile(1, aGmemTile.elementsPerLDG).to(Lane).donePtx
      ).align(FP16.bitWidth).guard(s"${test(Var("SPLIT"))} < (KK / ${ctaTile.k})")
      .load(MatMul.a, SH, Fluent
        .tile(aGmemTile.columnsPerLDG, aGmemTile.contiguous).unrollTile
        .tile(aGmemTile.columnsPerLDGPerWarp, aGmemTile.contiguous).to(Warp)
        .tile(1, aGmemTile.elementsPerLDG).to(Lane)
        .swizzle(stsSwizzle) //.printSwizzle(stsSwizzleScala)
        .done
      ).noSync.postponed
      //--- B: GL -> SH ------------------------------------------------------------------
      .load(MatMul.b, RF, Fluent
        .tile(bGmemTile.contiguous, bGmemTile.columnsPerLDG).unrollTile
        .tile(bGmemTile.contiguous, bGmemTile.columnsPerLDGPerWarp).to(Warp)
        .tile(bGmemTile.elementsPerLDG, 1).to(Lane).threadLayout(ThreadLayout.ColMajor).donePtx
      ).align(FP16.bitWidth).guard(s"${test(Var("SPLIT"))} < (KK / ${ctaTile.k})")
      .load(MatMul.b, SH, Fluent
        .tile(bGmemTile.contiguous, bGmemTile.columnsPerLDG).unrollTile
        .tile(bGmemTile.contiguous, bGmemTile.columnsPerLDGPerWarp).to(Warp)
        .tile(bGmemTile.elementsPerLDG, 1).to(Lane).threadLayout(ThreadLayout.ColMajor)
        .swizzle(stsSwizzle) //.printSwizzle(stsSwizzleScala)
        .done
      ).postponed
      /// WARP-level /////////////////////////////////////////////////////////////////////
      .tile(warpTileM, warpTileN).to(Warp)
      //--- XMMA-tile ------------------------------------------------------------------//
      .split(8).unrollSplit.vars("XMMAS_K").swizzle(ldsASwizzle, ldsBSwizzle).doubleBufferLoop
      .load(MatMul.a, RF, loadAFragments).doubleBuffer
      .load(MatMul.b, RF, loadBFragments).doubleBuffer
      .tile(16, 16).unrollTile.vars("XMMAS_N", "XMMAS_M")
      //--- _mma-tile ------------------------------------------------------------------//
      /// LANE-level /////////////////////////////////////////////////////////////////////
      .mma // implicitly assigns created chunks to lanes
      .done\end{lstlisting}
\caption{Fireiron: HMMA similar to XMMA.}
\label{fig:splitk}
\end{figure*}

\subsection{XMMA Comparison}
\begin{figure*}
    \includegraphics[width=\linewidth]{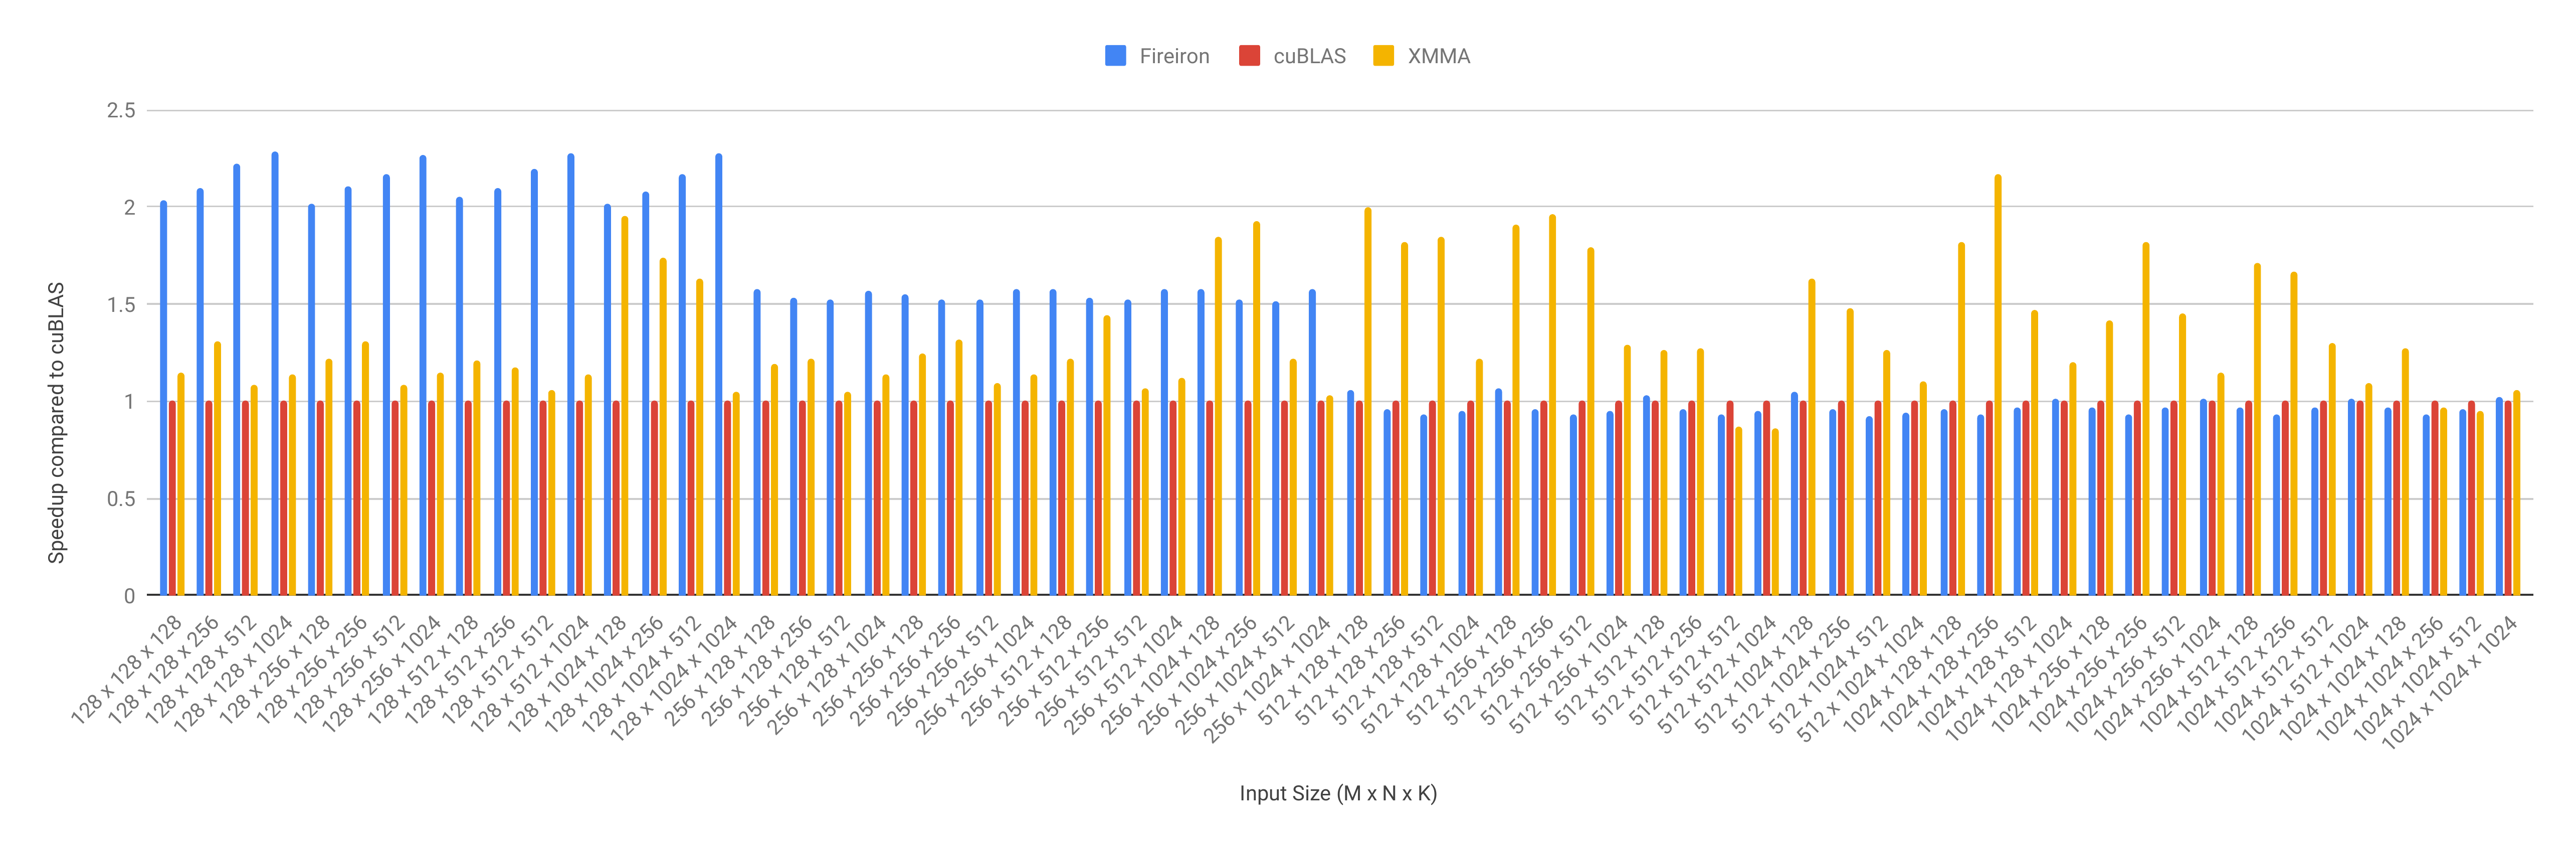}
        \caption{todo}
        \label{fig:small-matrices2}
\end{figure*}
\begin{figure}
    \includegraphics[width=\linewidth]{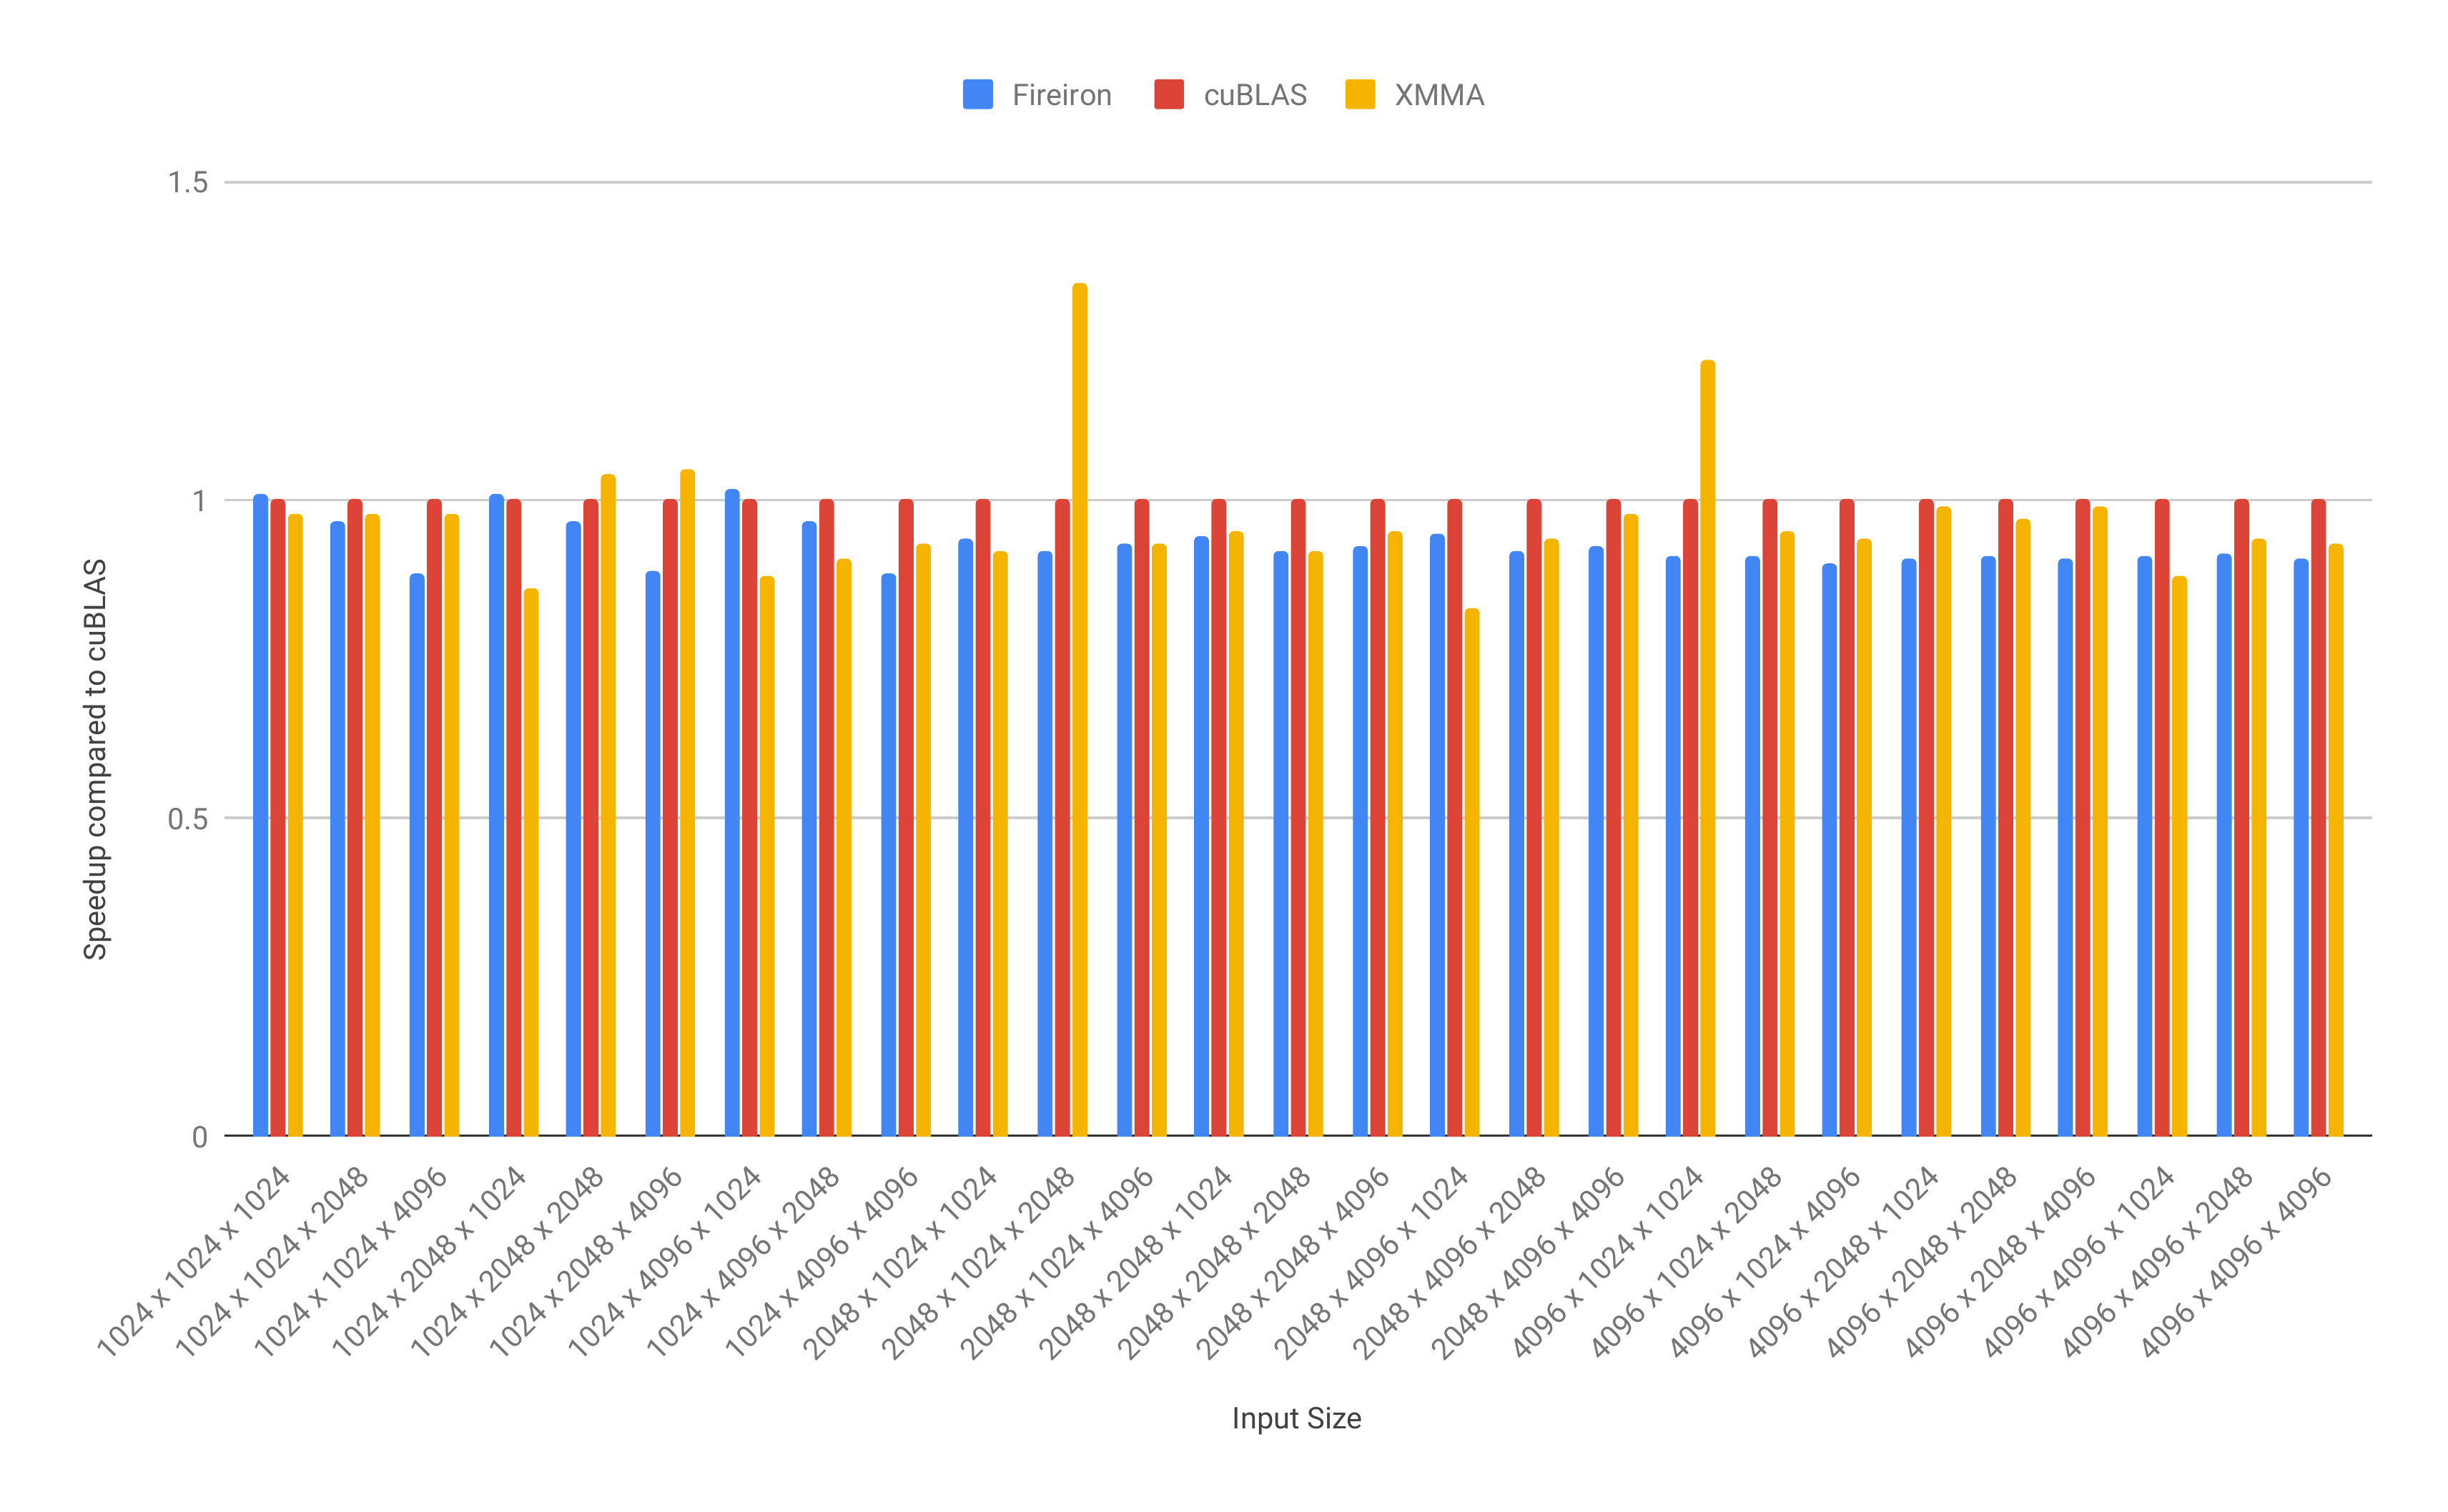}
        \caption{todo}
        \label{fig:large-matrices2}
\end{figure}
